# Supplementary material for: KernelBench: Can LLMs Write Efficient GPU Kernels?
Source: arXiv:2502.10517 source file (2025-02-14)
Supplement: Supplementary file 2 [file multi-turn-analysis.tex]

We show trajectories in multi-turn.
